# Supplementary material for: Breakup of particle-laden droplets in airflow
Source: arXiv:2310.04273 source file (2023-10-06)
Supplement: Supplementary file 1 [file SM.pdf]

# Breakup of particle-laden droplets in airflow: Supplementary material

Zhikun Xu<sup>1</sup>, Tianyou Wang<sup>1,2</sup> and Zhizhao Che<sup>1,2†</sup>

<sup>1</sup>State Key Laboratory of Engines, Tianjin University, Tianjin 300350, China

<sup>2</sup>National Industry-Education Platform of Energy Storage, Tianjin University, Tianjin 300350, China

(6 October 2023)

## 1. Image processing details for the measurement of fragment sizes

The droplet breakup is a continuous process with different parts breaking up at different moments. After the completion of the droplet breakup, the fragments are already dispersed to a large region. To maintain sufficient spatial resolution for the large region, we used two cameras to shoot different parts, as shown in figures S1 and S2 for low-order multimode breakup and bag breakup, respectively. By combining the images from the two cameras, we can obtain all fragments larger than 0.2 mm. As shown in figure S2, most of the fragments are measured. Only very small fragments are removed to ensure the accuracy of the reported results, and this fraction only occupies a very small volume of the overall fragments. The measurement results based on the present resolution can clearly show the changes in the shape and position of different peaks, which reflects the effects of particles on the sizes of fragments produced by the main structures of the droplet (including the bag, the ring, and the nodes). For the smallest fragments considered, the uncertainty of the fragment size caused by the image resolution is about  $\pm 15\%$  ( $200 \pm 30 \mu\text{m}$ ). For fragments size corresponding to different peaks, the uncertainties are about  $\pm 6\%$  ( $500 \pm 30 \mu\text{m}$ ) for the first peak,  $\pm 3\%$  ( $1000 \pm 30 \mu\text{m}$ ) for the second peak, and  $\pm 1.9\%$  ( $1600 \pm 30 \mu\text{m}$ ) for the third peak, respectively.

The typical images from which the sizes are obtained are shown in figures S1(*a*, *b*) and S2(*a*, *b*). For each image, we performed digital image processing to obtain the fragment size. We first removed the background of the raw images by subtracting an image without any droplets. Then the image was binarized based on a threshold in the brightness, and the holes in the middle of the fragments in the binary image were filled. After that, objects smaller than 9 pixels were removed from the binary image, as they have a large error in calculating the fragment size. The areas of the objects in pixels *S* were obtained from the image by region analysis and then converted to the surface equivalent fragment size *d* by using a scale factor *c* obtained from a calibration image, which is achieved by

† Email address for correspondence: chezhizhao@tju.edu.cn

$d = 2c\sqrt{S/\pi}$ . As shown in figures S1( $c, d$ ) and S2( $c, d$ ), the fragments highlighted by the green circles in the two images include all considered fragments.

In addition, the circularities of all considered fragments were extracted through digital image processing. As shown in figure S3( $a, b$ ), the circularities of most of the fragments are close to 1, indicating that most of the fragments are almost spherical. Similar to Wang & Bourouiba (2018), we extract the time evolution of some fragment sizes based on the projected area. As shown in figure S3( $c, d$ ), different plots correspond to different fragments, and the corresponding fragments are marked by yellow dashed circles in figures S1 and S2. For the multimode breakup (figure S1), most of the fragment sizes have been stabilized (such as fragments 1–4 in figure S3( $c$ )), and only a few fragments are still oscillating (such as fragment 5 in figure S3( $c$ )). This is unavoidable because under the multimode breakup mode, the airflow velocity is fast and the fragments spread quickly to a large region. To capture all fragments, the fragment sizes are measured when a few fragments are still oscillating. In our measurements, we usually select images where all fragments reach spherical shapes and the images can capture all fragments. Moreover, for the bag breakup (figure S2), almost all the fragments are spherical (shown in figure S3( $b$ )) and their sizes have stabilized (shown in figure S3( $d$ )). This is because the airflow velocity is slow relatively under the bag breakup mode and almost all fragments have time to reach a spherical shape.

## REFERENCES

- WANG, Y. & BOUROUBA, L. 2018 Unsteady sheet fragmentation: droplet sizes and speeds. *Journal of Fluid Mechanics* **848**, 946–967.

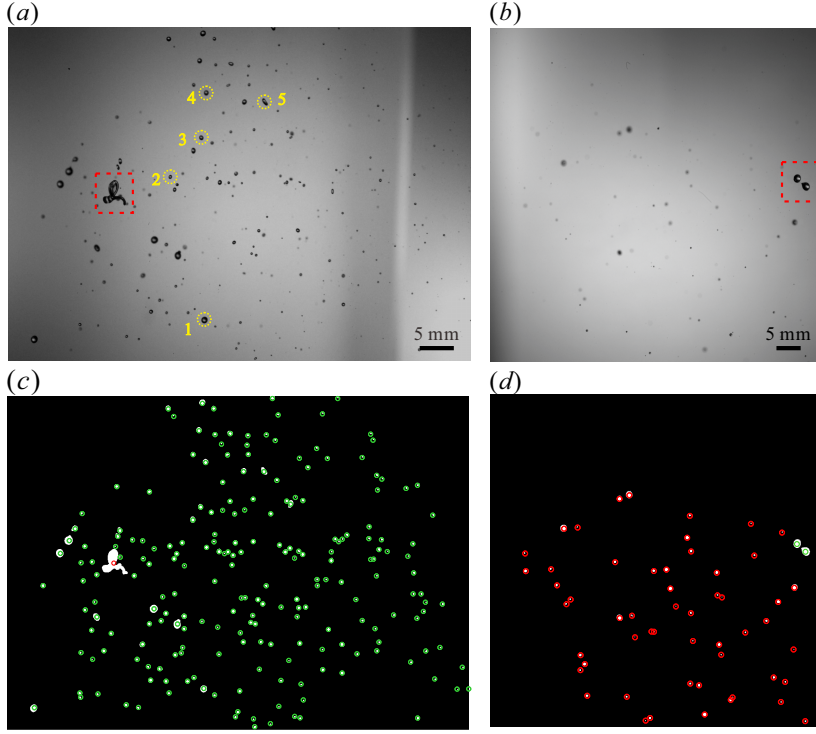

FIGURE S1. Measurement of fragment size from different images in the low-order multimode breakup. *(a, c)* Raw and binary images obtained from the upstream camera, mainly for calculating the fragments of the peripheral nodes and peripheral ring. *(b, d)* Raw and binary images obtained from the downstream camera, mainly for calculating the fragments of the middle node (corresponding to the part in the red box). The fragments highlighted by the green circles in *(c, d)* include all considered fragments. The sizes of the fragments highlighted by the yellow dashed circles in *(a)* are measured over time in figure S3(c).

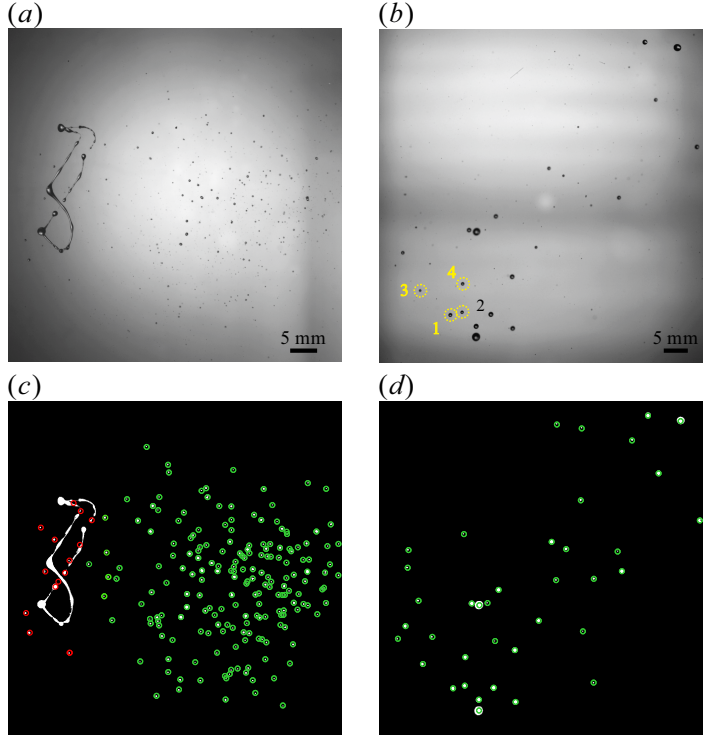

FIGURE S2. Measurement of fragment size from different images in the bag breakup. *(a, c)* Raw and binary images obtained from the upstream camera, mainly for calculating the fragments of the bag film. *(b, d)* Raw and binary images obtained from the downstream camera, mainly for calculating the fragments of the node and the ring. The fragments highlighted by the green circles in *(c, d)* include all considered fragments. The sizes of the fragments highlighted by the yellow dashed circles in *(b)* are measured over time in figure S3(*d*).

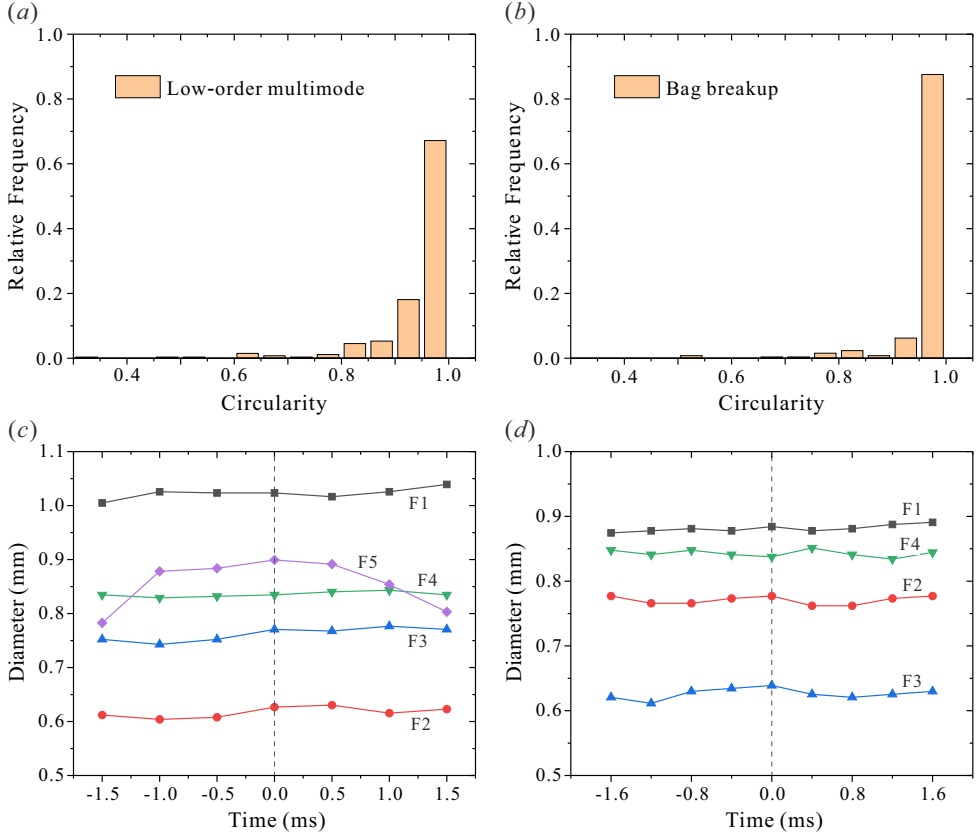

FIGURE S3. (a, b) Circularity of the fragments considered in figures S1 and S2. (c, d) Time evolution of sizes of some fragments marked by yellow dashed circles in figures S1(a) and S2(b). (a, c) correspond to the low-order multimode breakup, (b, d) correspond to the bag breakup.
